# Supplementary material for: Many-body eigenstate thermalization from one-body quantum chaos: emergent arrow of time
Source: arXiv:1606.08371 source file (2016-06-24)
Supplement: Supplementary file 1 [file thermalization_SM.pdf]

# Supplementary Material

## I. Evolution of correlation function

### I.1. Evolution equation

The initial state evolves in time, $F \to F(t)$, following

$$i\hbar\partial_t|F(t)\rangle = \hat{H}_{tot.}|F(t)\rangle, \tag{S1}$$

with $\hat{H}_{tot.} \equiv \sum_{i=1}^N H(\hat{\boldsymbol{q}}_i, \hat{\boldsymbol{p}}_i)$ being the total Hamiltonian and $|F(0)\rangle \equiv |F\rangle$. Solving Eq. (S1) we obtain

$$|F(t)\rangle = \sum_{\boldsymbol{m}} e^{-iE_{\boldsymbol{m}}t/\hbar} C_{\boldsymbol{m}}|\boldsymbol{m}\rangle, \tag{S2}$$

where the (many-body) eigenenergy

$$E_{\boldsymbol{m}} = \sum_\nu n_\nu \varepsilon_\nu, \tag{S3}$$

corresponding to eigenstate $|\boldsymbol{m}\rangle = |\{n_\nu\}\rangle$, is located inside a narrow energy window. Substituting Eqs. (S2) and (S3) into the definition of correlation function, we obtain

$$M_{\boldsymbol{r}\boldsymbol{r}'}(t) = \sum_{\nu'\nu} C_{\nu'\nu}\psi_{\nu'}(\boldsymbol{r})\psi^*_\nu(\boldsymbol{r}')e^{-i(\varepsilon_{\nu'}-\varepsilon_\nu)t/\hbar}, \tag{S4}$$

with the coefficient

$$\begin{aligned} C_{\nu'\nu} &= \sum_{\boldsymbol{m}\boldsymbol{m}'} C^*_{\boldsymbol{m}}C_{\boldsymbol{m}'}\sqrt{n_\nu n'_{\nu'}}(\mp)^{\sum_{\mu'<\nu'}n_{\mu'}-\sum_{\mu<\nu}n'_\mu} \\ &\quad\times\Big((1-\delta_{\nu,\nu'})\delta_{n_\nu,n'_\nu+1}\delta_{n_{\nu'},n'_{\nu'}-1}\prod_{\mu\neq\nu,\nu'}\delta_{n_\mu,n'_\mu} \\ &\quad+\delta_{\nu,\nu'}\prod_\mu \delta_{n_\mu,n'_\mu}\Big). \end{aligned} \tag{S5}$$

Recall that the upper (lower) sign corresponds to the Fermi (Bose) statistics. Equation (S4) is a solution to the von Neumann equation,

$$\partial_t\hat{M}(t) = -\frac{i}{\hbar}[H(\hat{\boldsymbol{q}},\hat{\boldsymbol{p}}),\hat{M}(t)], \tag{S6}$$

where $\hat{M} \equiv \{M_{\boldsymbol{r}\boldsymbol{r}'}\}$. Note that here $H(\hat{\boldsymbol{q}},\hat{\boldsymbol{p}})$ is single-particle Hamiltonian.

### I.2.Quantum recurrence

Because $N$ is finite the right-hand side of Eq. (S4) is a finite sum. In other words, the dimension of the Hilbert space supporting the evolution of $M_{\boldsymbol{r}\boldsymbol{r}'}(t)$ is finite. According to a general theorem [1], the evolution of $M_{\boldsymbol{r}\boldsymbol{r}'}(t)$ exhibits quantum recurrence. In this part we estimate the recurrent time $t_{rec.}$ by generalizing the method of Peres [2]. For simplicity we focus on Fermi gas.

When the recurrence occurs the matrix $\hat{M}(t)$ is arbitrarily close to its initial value, i.e.,

$$\|\hat{M}(t) - \hat{M}(0)\| \le \epsilon, \tag{S7}$$

where $\epsilon$ is an arbitrarily small positive number. With the substitution of Eq. (S4) this reduces to

$$\begin{aligned} &\|\hat{M}(t) - \hat{M}(0)\| \\ &= 4\sum_{\nu\neq\nu'}|C_{\nu\nu'}|^2\sin^2\frac{(\varepsilon_\nu-\varepsilon_{\nu'})t}{2\hbar} \le \epsilon. \end{aligned} \tag{S8}$$

The value of $|C_{\nu\nu'}|^2$ can be estimated as follows. We assume that all $\boldsymbol{m}$s in initial state $F$ are typical, realized via random occupation of single-particle eigenenergies, which gives $|C_{\boldsymbol{m}}| = \frac{1}{\sqrt{C_M^N}}$ with $M(\gg N)$ being the number of available single-particle energies. Using the definition (S5) of $C_{\nu\nu'}$, we obtain

$$|C_{\nu\nu'}|^2 = \left(C_{M-2}^{N-1}/C_M^N\right)^2 \approx (N/M)^2. \tag{S9}$$

On the other hand, the inequality (S8) implies that all phases, $\frac{(\varepsilon_\nu-\varepsilon_{\nu'})t}{2\hbar}$, are closed to multiple $\pi$, i.e.,

$$\sum_{\nu\neq\nu'}\left(\frac{(\varepsilon_\nu-\varepsilon_{\nu'})t}{2\pi\hbar} - k_{\nu\nu'}\right)^2 \le \left(\frac{M}{2\pi N}\right)^2\epsilon \tag{S10}$$

with $k_{\nu\nu'} \in \mathbb{Z}$. The equality defines a sphere,

$$\sum_{\nu\neq\nu'}\left(\frac{(\varepsilon_\nu-\varepsilon_{\nu'})t}{2\pi\hbar} - x_{\nu\nu'}\right)^2 = \left(\frac{M}{2\pi N}\right)^2\epsilon \tag{S11}$$

centered at $\{\frac{(\varepsilon_\nu-\varepsilon_{\nu'})t}{2\pi\hbar}\}$ in $M(M-1)/2$-dimensional space and of radius $\frac{M\sqrt{\epsilon}}{2\pi N}$. The cross section of the sphere is

$$\sigma \equiv \frac{\pi^{\frac{M(M-1)/2-1}{2}}\left(\frac{M\sqrt{\epsilon}}{2\pi N}\right)^{M(M-1)/2-1}}{\Gamma\left(\frac{M(M-1)/2+1}{2}\right)}. \tag{S12}$$

The center moves in the course of time with a constant "velocity" of $\{\frac{(\varepsilon_\nu-\varepsilon_{\nu'})}{2\pi\hbar}\}$. In a duration of $t$ the cross section of the sphere transverse to the velocity sweeps a cylinder. At $t = t_{rec.}$ this cylinder includes a lattice point $\{k_{\nu\nu'}\}$. This gives

$$\left(\frac{M(M-1)}{2}\right)^{1/2}\frac{\Delta\varepsilon}{2\pi\hbar}\sigma t_{rec.} = 1, \tag{S13}$$

where $\Delta\varepsilon$ is the mean squared value of $(\varepsilon_\nu - \varepsilon_{\nu'})$. As a result,

$$t_{rec.} \sim \frac{\hbar}{\Delta\varepsilon}\frac{1}{M}\left(\frac{N}{\sqrt{\epsilon}}\right)^{\frac{M^2}{2}} \gg \frac{\hbar}{\Delta\varepsilon}\frac{1}{N}\left(\frac{N}{\sqrt{\epsilon}}\right)^{\frac{N^2}{2}}. \tag{S14}$$

This shows that the recurrent time is extremely large for $N \gg 1$ and the recurrence phenomenon can be ignored practically.

### I.3. Evolution in Wigner representation

Passing to the Wigner representation, $H(\hat{\boldsymbol{q}}, \hat{\boldsymbol{p}}) \to H(\boldsymbol{q}, \boldsymbol{p})$ and $M_{\boldsymbol{r}\boldsymbol{r}'}(t) \to M(\boldsymbol{q}, \boldsymbol{p}; t)$, we follow the standard procedure [3] and reduce Eq. (S6) to Eq. (6). For $t > 0$ the latter is solved by

$$M(t) = G(t) \circ M(0). \tag{S15}$$

Here $M(t)$ is the shorthand notation of $M(\boldsymbol{q}, \boldsymbol{p}; t)$ and $G(t)$ of $G(\boldsymbol{q}, \boldsymbol{p}, \boldsymbol{q}', \boldsymbol{p}'; t)$. The latter is the Green's function of the Moyal equation [4],

$$\begin{aligned} &(\partial_t - \{H(\boldsymbol{q}, \boldsymbol{p}), \cdot\}_{\text{Moyal}})\, G(\boldsymbol{q}, \boldsymbol{p}, \boldsymbol{q}', \boldsymbol{p}'; t) \\ &= \delta(\boldsymbol{q} - \boldsymbol{q}')\delta(\boldsymbol{p} - \boldsymbol{p}')\delta(t). \end{aligned} \tag{S16}$$

The $\circ$-product is defined as

$$(A \circ B)(\boldsymbol{q}, \boldsymbol{p}) \equiv \iint d\boldsymbol{q}' d\boldsymbol{p}' A(\boldsymbol{q}, \boldsymbol{p}, \boldsymbol{q}', \boldsymbol{p}') B(\boldsymbol{q}', \boldsymbol{p}'), \tag{S17}$$

and has an important property,

$$(A \circ B) \circ C = A \circ (B \circ C). \tag{S18}$$

For $t < 0$ the solution can be found in a similar way.

To proceed further we also introduce the Green's function, $\mathcal{G}(\boldsymbol{q}, \boldsymbol{p}, \boldsymbol{q}', \boldsymbol{p}'; t)$, of the Liouville equation, defined as

$$\begin{aligned} &(\partial_t - \{H(\boldsymbol{q}, \boldsymbol{p}), \cdot\})\, \mathcal{G}(\boldsymbol{q}, \boldsymbol{p}, \boldsymbol{q}', \boldsymbol{p}'; t) \\ &= \delta(\boldsymbol{q} - \boldsymbol{q}')\delta(\boldsymbol{p} - \boldsymbol{p}')\delta(t). \end{aligned} \tag{S19}$$

With the help of this auxiliary Green's function we can rewrite Eq. (S16) as

$$\begin{aligned} G(t) &= \mathcal{G}(t) + \int dt' \mathcal{G}(t - t') \\ &\quad \circ (\{H, \cdot\}_{\text{Moyal}} - \{H, \cdot\}) \circ G(t'), \end{aligned} \tag{S20}$$

where

$$\begin{aligned} &\{H, \cdot\}_{\text{Moyal}} - \{H, \cdot\} \\ &= \sum_{n=1}^{\infty} \frac{(-\hbar^2)^n}{(2n+1)!} V(\boldsymbol{q}) (\overleftarrow{\partial}_{\boldsymbol{q}} \cdot \overrightarrow{\partial}_{\boldsymbol{p}})^{2n+1} (\cdot). \end{aligned} \tag{S21}$$

By iteration we find that the solution of $G(t)$ is highly singular. Mathematically, $G(t)$ is not a function, but, a distribution or generalized function [5]. What is physically important is that, with its substitution into Eq. (S15), $M(\boldsymbol{q}, \boldsymbol{p}; t)$ exhibits more and more rapid oscillations in phase space coordinates as the time increases. From the iteration solution of Eq. (S20) it is clear that the evolution of $G(\boldsymbol{q}, \boldsymbol{p}, \boldsymbol{q}', \boldsymbol{p}'; t)$ is restricted on the energy shell of (single-particle) phase space, i.e., $G(\boldsymbol{q}, \boldsymbol{p}, \boldsymbol{q}', \boldsymbol{p}'; t)$ is a functional of $\delta(H(\boldsymbol{q}, \boldsymbol{p}) - H(\boldsymbol{q}', \boldsymbol{p}'))$. Therefore, the oscillatory structures exhibited by $M(\boldsymbol{q}, \boldsymbol{p}; t)$ are developed on the energy shell.

### I.4. Evolution of $M_{c.g.}(t)$ and relation to classical irreversibility

As discussed in the paper, the definition of $\overline{M_{\boldsymbol{r}\boldsymbol{r}'}(t)}$ [cf. Eq. (5)] essentially introduces the coarse graining of the phase space energy shell. To implement this coarse graining we replace the Dirac distribution $\delta(\boldsymbol{q} - \boldsymbol{q}')\delta(\boldsymbol{p} - \boldsymbol{p}')$ by

$$\begin{aligned} &\chi(\boldsymbol{q}, \boldsymbol{p}, \boldsymbol{q}', \boldsymbol{p}') \\ &\equiv \chi'(\boldsymbol{q}, \boldsymbol{p}, \boldsymbol{q}', \boldsymbol{p}') \delta(H(\boldsymbol{q}, \boldsymbol{p}) - H(\boldsymbol{q}', \boldsymbol{p}')), \end{aligned} \tag{S22}$$

where $\chi'$ is a smooth function on the energy shell with compact support. The details of $\chi'$ are irrelevant for present discussions. Then, we multiply – in the sense of $\circ$-product – both sides of Eq. (S15) by $\chi$ from the left. With the help of Eqs. (S18) and (S20), we obtain

$$\begin{aligned} M_{c.g.}(t) &= M_{cl.}(t) + \int dt' \chi \circ \mathcal{G}(t - t') \\ &\quad \circ (\{H, \cdot\}_{\text{Moyal}} - \{H, \cdot\}) \circ M(t'). \end{aligned} \tag{S23}$$

Here,

$$M_{c.g.}(t) \equiv \chi \circ M(t) \tag{S24}$$

is the local phase space average of the Wigner function $M(\boldsymbol{q}, \boldsymbol{p}; t)$, and

$$M_{cl.}(t) \equiv \chi \circ \mathcal{G}(t) \circ M(0) \tag{S25}$$

of $\mathcal{G}(t) \circ M(0)$. The latter Wigner function follows the Liouville equation, and the subscript '*cl.*' implies its purely classical evolution nature. Note that

$$\iint d\boldsymbol{q} d\boldsymbol{p} M_{c.g.}(\boldsymbol{q}, \boldsymbol{p}; t) = \iint d\boldsymbol{q} d\boldsymbol{p} M(\boldsymbol{q}, \boldsymbol{p}; t). \tag{S26}$$

In addition, the coarse graining does not violate the unitarity of quantum evolution $M(t)$.

Because the classical flow in phase space conserves the volume (namely Lebesgue measure), Eq. (S23) can be rewritten as

$$\begin{aligned} M_{c.g.}(t) &= M_{cl.}(t) + \int dt' \left( e^{-(t-t')\{H, \cdot\}} \chi \right) \\ &\quad \circ (\{H, \cdot\}_{\text{Moyal}} - \{H, \cdot\}) \circ M(t'). \end{aligned} \tag{S27}$$

Here $e^{-t\{H, \cdot\}}$ is the Perron-Frobenius operator [6], which plays central roles in classical nonequilibrium statistical mechanics notably in studies of classical irreversibility [7–9]. Therefore, the Liouville evolution of phase space density, i.e.,

$$e^{-(t-t')\{H, \cdot\}} \chi', \tag{S28}$$

as well as the first term $M_{cl.}(t)$ of Eq. (S27) determined by Eqs. (S19) and (S25) establishes a rigorous connection between classical irreversibility and quantum evolution $M(t)$.

### I.5. Short-time evolution of $M_{c.g.}(t)$

To study the evolution of $M_{c.g.}(t)$ at short times, i.e., $t \ll t_E$, it is more convenient to use Eqs. (S15) and (S20) as well as the definition (S24). Specifically, we iterate Eq. (S20) and substitute the result into Eqs. (S15) and (S24). This gives an expansion in $(\{H,\cdot\}_{\rm Moyal}-\{H,\cdot\})$. By using Eq. (S21), we find

$$e^{t\{H,\cdot\}}\left(\{H,\cdot\}_{\rm Moyal}-\{H,\cdot\}\right)e^{-t\{H,\cdot\}} = \sum_{n=1}^{\infty} e^{2n\lambda(t-t_E)}\mathcal{O}\left(V(\boldsymbol{q})\overleftarrow{\partial}_{\boldsymbol{q}}\cdot\overrightarrow{\partial}_{\boldsymbol{p}}\right)(\cdot). \qquad \text{(S29)}$$

Here the exponential arises from one-body quantum chaos, as discussed in the paper. Because of $e^{\lambda(t-t_E)} \ll 1$, we can ignore all the higher order expansions in $(\{H,\cdot\}_{\rm Moyal}-\{H,\cdot\})$. This gives

$$M_{c.g.}(t) \approx M_{cl.}(t), \quad \text{for}\, t \ll t_E. \qquad \text{(S30)}$$

In words, the evolution of $M_{c.g.}(t)$ is classical in short times.

### I.6. Long-time evolution of $M_{c.g.}(t)$

Now we turn to the opposite limit, $t \gg t_E$. In this case, we need to sum up the entire series of expansion in $(\{H,\cdot\}_{\rm Moyal}-\{H,\cdot\})$ due to $e^{\lambda(t-t_E)} \gg 1$. This is an intractable task. To deal with this non-perturbative regime we return to Eq. (S27).

We note that, for mixing (actually, more sophisticated conditions, as those defining Axiom A systems [8–10], are required) systems, the evolution governed by the Perron-Frobenius operator leads to exponential decay of correlation of generic observables in time [8, 9]. This implies that an initial density (not the Dirac distribution) on the energy shell relaxes to an invariant density which is uniform, according to

$$e^{-t\{H,\cdot\}}\chi' = 1 + \sum_{n=1}^{\infty} e^{-\gamma_n t} c_n \chi_n. \qquad \text{(S31)}$$

Here, $\{\gamma_n\}$ (Re$\gamma_n > 0$) are the so-called Ruelle-Pollicott resonances [8, 9], i.e., the poles of the reolvent of the Liouville operator $\{H,\cdot\}$, $\{\chi_n\}$ the corresponding eigendistributions, and $\{c_n\}$ the expansion coefficients.

Then, we divide the $t'$-integral in Eq. (S27) into two parts, i.e.,

$$\int dt' \equiv \int_0^t dt' = \int_{t-1/{\rm Re}\gamma_1}^t dt' + \int_0^{t-1/{\rm Re}\gamma_1} dt' \qquad \text{(S32)}$$

where $\gamma_1$ is the leading resonance and $1/{\rm Re}\gamma_1 \lesssim t_E$, and consider two integrals separately:

- For the first integral, the factor $e^{-(t-t')\{H,\cdot\}}\chi'$ in the integrand does not lead to relaxation of $\chi'$ because of $(t-t'){\rm Re}\gamma_1 \le 1$. [Note that the Liouville evolution has no consequences on $\delta(H(\boldsymbol{q},\boldsymbol{p})-H(\boldsymbol{q}',\boldsymbol{p}'))$ in the definition (S22).] Therefore, this factor gives a smooth function in phase space with compact support (slightly deformed from $\chi'$). On the other hand, as discussed in the paper fine quantum structures exhibited by $M(t)$ are formed at $t \gtrsim t_E$ (cf. Fig. 1). Thanks to $t' > t - 1/{\rm Re}\gamma_1 \gg t_E$ the function $(\{H,\cdot\}_{\rm Moyal}-\{H,\cdot\})\circ M(t')$ oscillates rapidly in a scale much smaller than the scale over which $e^{-(t-t')\{H,\cdot\}}\chi'$ varies. With the phase space integral carried out, the integrand gives a negligibly small result.
- For the second integral, with the substitution of Eq. (S31) into the integrand we find that $e^{-(t-t')\{H,\cdot\}}\chi' = 1$ because of $(t-t'){\rm Re}\gamma_1 \ge 1$. So, the integrand is simplified to $1\circ(\{H,\cdot\}_{\rm Moyal}-\{H,\cdot\})\circ M(t')$. For $t' \le t_E$, the evolution of $M(t')$ is (largely) classical and $M(t')$ decays to zero in the boundary of momentum ($\boldsymbol{p}$) space. This gives a vanishing integrand, since the latter includes a $\boldsymbol{p}$-integral and this integral is separated from the spatial ($\boldsymbol{q}$-) integral [cf. Eq. (S21)]. For $t_E \le t' \le t - 1/{\rm Re}\gamma_1$, fine quantum structures develop and $M(t')$ oscillates rapidly in phase space coordinates. This gives a vanishing integrand again.

Taking analyses above into account we find that the second term of Eq. (S27) vanishes, giving

$$M_{c.g.}(t) \overset{t\gg t_E}{\to} M_{cl.}(t). \qquad \text{(S33)}$$

It should be emphasized that, different from Eq. (S30), this is a highly nonperturbative result.

To find the right-hand side of Eq. (S33) we rewrite Eq. (S25) as

$$M_{cl.}(t) = \left(e^{-t\{H,\cdot\}}\chi\right)\circ M(0). \qquad \text{(S34)}$$

Substituting Eq. (S31) into it we obtain

$$M_{cl.}(\boldsymbol{q},\boldsymbol{p};t) = \iint d\boldsymbol{q}'d\boldsymbol{p}'\delta(H(\boldsymbol{q},\boldsymbol{p})-H(\boldsymbol{q}',\boldsymbol{p}'))M(\boldsymbol{q}',\boldsymbol{p}';0) \qquad \text{(S35)}$$

for $t \gg t_E$. This is essentially the average of $M(0)$ with respect to the *single-particle* microcanonical distribution. Therefore, this average is a function of $H(\boldsymbol{q},\boldsymbol{p})$ and uniform on the energy shell. In combination with Eq. (S33), we find

$$M_{c.g.}(\boldsymbol{q},\boldsymbol{p};t) \overset{t\gg t_E}{\to} \iint d\boldsymbol{q}'d\boldsymbol{p}'\delta(H(\boldsymbol{q},\boldsymbol{p})-H(\boldsymbol{q}',\boldsymbol{p}'))M(\boldsymbol{q}',\boldsymbol{p}';0). \qquad \text{(S36)}$$

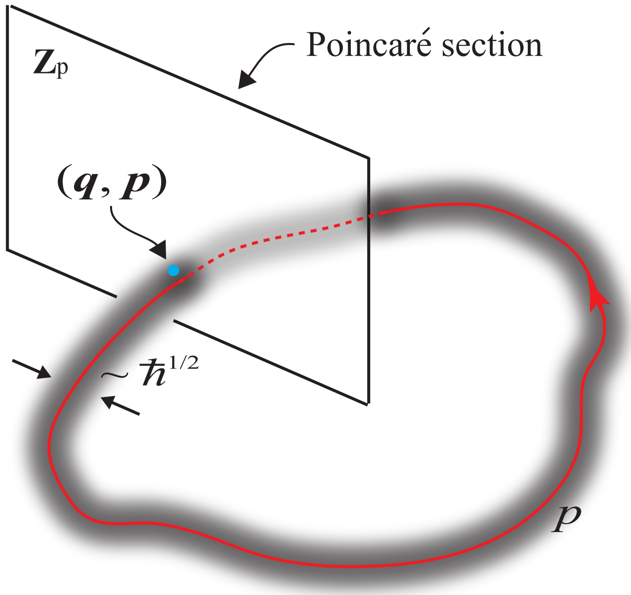


FIG. S1: The quantum scar (thick grey line) passing through the vicinity of the phase point $(\boldsymbol{q}, \boldsymbol{p})$ is a fringe pattern of width $\sim \hbar^{1/2}$ decorating a classical periodic orbit $p$ (red line), superimposing on the microcanonical distribution in the energy shell. The fuzzyness of the orbit by quantum uncertainty is characterized by the extension of the pattern in the Poincaré section transverse to the orbit.

## II. Effects of quantum scars

For a classical chaotic system, there are periodic orbits labeled by $p$. These orbits are typically isolated, which we shall assume below for simplicity. The purpose of this section is to show that these orbits, though of non-ergodic nature, have no influences on quantum thermalization for $E/N$ much larger than the mean level spacing.

In the classical limit, a periodic orbit is a zero measure set invariant under the Liouville evolution. Semiclassically, each periodic orbit can be resolved to certain degree. Loosely speaking, it acquires a finite thickness (cf. Fig. S1) as a result of quantum uncertainty. Formally, each periodic orbit contributes an oscillatory correction which superimposes on the microcanonical distribution (9), i.e.,

$$\overline{\Psi_\nu(\boldsymbol{q},\boldsymbol{p})} \to \frac{\delta(\varepsilon - H(\boldsymbol{q},\boldsymbol{p}))}{\iint d\boldsymbol{q}d\boldsymbol{p}\delta(\varepsilon - H(\boldsymbol{q},\boldsymbol{p}))} \times \left(1 + \sum_p A_p e^{\frac{i}{\hbar}S_p + i\gamma_p\frac{\pi}{4}} e^{\frac{i}{\hbar}\mathbf{Z}_p\cdot\mathbf{W}_p\cdot\mathbf{Z}_p}\right). \quad \text{(S37)}$$

Here, the sum is over all periodic orbits on the energy (i.e., $\varepsilon$ corresponding to the eigenfunction $\psi_\nu$) shell in single-particle phase space. $S_p$ is the action of the orbit $p$. $\mathbf{Z}_p$ are the $2(d-1)$ coordinates of the Poincaré section which is transverse to the orbit (see Fig. S1 for illustrations). $\gamma_p$, $A_p$ and $\mathbf{W}_p$ are completely determined by the monodromy matrix characterizing the instability of the orbit. Their details, except being $\hbar$ independent, are unimportant for present discussions. This is the so-called quantum scar [11, 12] in phase space [13]. Equation (S37) shows that it has a thickness $\sim \mathcal{O}(\hbar^{1/2})$ in the semiclassical regime.

With the help of Eq. (S37), we obtain

$$\overline{C_\nu(\boldsymbol{r}-\boldsymbol{r}',\boldsymbol{q})} \to \frac{\int d\boldsymbol{p} e^{-\frac{i}{\hbar}(\boldsymbol{r}-\boldsymbol{r}')\cdot\boldsymbol{p}}\delta(\varepsilon - H(\boldsymbol{q},\boldsymbol{p}))}{\iint d\boldsymbol{q}d\boldsymbol{p}\delta(\varepsilon - H(\boldsymbol{q},\boldsymbol{p}))} + \overline{\delta C_\nu(\boldsymbol{r}-\boldsymbol{r}',\boldsymbol{q})}. \quad \text{(S38)}$$

[Note that to invoke Eq. (S37) we have to make the boundary be a soft potential. This does not affect physics qualitatively.] The correction arising from quantum scars is

$$\begin{aligned} &\overline{\delta C_\nu(\boldsymbol{r}-\boldsymbol{r}',\boldsymbol{q})} \\ &= \left(\iint d\boldsymbol{q}d\boldsymbol{p}\delta(\varepsilon - H(\boldsymbol{q},\boldsymbol{p}))\right)^{-1} \int d\boldsymbol{p}\delta(\varepsilon - H(\boldsymbol{q},\boldsymbol{p})) \\ &\quad \times e^{-\frac{i}{\hbar}(\boldsymbol{r}-\boldsymbol{r}')\cdot\boldsymbol{p}} \sum_p A_p e^{\frac{i}{\hbar}S_p + i\gamma_p\frac{\pi}{4}} e^{\frac{i}{\hbar}\mathbf{Z}_p\cdot\mathbf{W}_p\cdot\mathbf{Z}_p} \\ &\sim \sum_p A_p e^{\frac{i}{\hbar}(\boldsymbol{r}_i-\boldsymbol{r}_j)\cdot\boldsymbol{p}_p(\boldsymbol{q})} e^{\frac{i}{\hbar}S_p + i\gamma_p\frac{\pi}{4}} \\ &\quad \times \int d\boldsymbol{\Omega} e^{\frac{i}{\lambda_\varepsilon}\left(-\boldsymbol{\Omega}\cdot(\boldsymbol{r}-\boldsymbol{r}') + \mathbf{Z}_p\cdot\frac{\mathbf{W}_p}{\sqrt{2m\varepsilon}}\cdot\mathbf{Z}_p\right)} \end{aligned} \quad \text{(S39)}$$

where the sum is over all the periodic orbits passing through the vicinity of $(\boldsymbol{q},\boldsymbol{p})$ with momentum $\boldsymbol{p}_p(\boldsymbol{q})$ (cf. Fig. S1). The last integral vanishes rapidly as $\lambda_\varepsilon \to 0$. So, the contribution of quantum scars to the autocorrelation of eigenfunction is negligible in the semiclassical regime. Using $\langle \boldsymbol{m}|a^\dagger_{\boldsymbol{r}'}a_{\boldsymbol{r}}|\boldsymbol{m}\rangle = \sum_\nu n_\nu C_\nu(\boldsymbol{r}-\boldsymbol{r}',\boldsymbol{q})$, we find that effects of quantum scars on the correlation function are negligible. In other words, they are harmless to thermalization when $E$ is sufficiently large.

We remark that the irrelevance of quantum scars to thermalization is consistent with a theoretical observation [14] that quantum scarring is intimately related to the Ruelle-Pollicott resonance. The thermalization deals with physics in long times, while the Ruelle-Pollicott resonance, as we have demonstrated in Sec. I.6, is important only in short times.

## III. Derivation of oscillation factor $f$

Without loss of generality we assume that $\boldsymbol{r}$ is in the $x_1$ direction, i.e., $\boldsymbol{r} = (r, 0, \cdots, 0)$. We parametrize the surface of a $d$-dimensional sphere, for which $\sum_{i=1}^d x_i^2 = 1$, by [15]

$$\begin{aligned} x_1 &= \cos\varphi_1, \\ x_2 &= \sin\varphi_1\cos\varphi_2, \\ x_3 &= \sin\varphi_1\sin\varphi_2\cos\varphi_3, \\ &\cdots\cdots\cdots\cdots\cdots \\ x_{d-1} &= \sin\varphi_1\sin\varphi_2\cdots\sin\varphi_{d-2}\cos\varphi_{d-1}, \\ x_d &= \sin\varphi_1\sin\varphi_2\cdots\sin\varphi_{d-2}\sin\varphi_{d-1}, \end{aligned} \quad \text{(S40)}$$

where

$$0 \le \varphi_1, \varphi_2, \cdots, \varphi_{d-2} \le \pi, \quad 0 \le \varphi_{d-1} < 2\pi. \quad \text{(S41)}$$

Correspondingly, the Jacobian

$$J = \sin^{d-2}\varphi_1 \sin^{d-3}\varphi_2 \cdots \sin^2\varphi_{d-3}\sin\varphi_{d-2}. \quad \text{(S42)}$$

Substituting Eqs. (S40)-(S42) into Eq. (11) we obtain

$$f\left(\frac{|\boldsymbol{r}-\boldsymbol{r}'|}{\lambda_\varepsilon}\right) = \frac{\int_0^\pi d\varphi_1 \sin^{d-2}\varphi_1 e^{-i\frac{|\boldsymbol{r}-\boldsymbol{r}'|}{\lambda_\varepsilon}\cos\varphi_1}}{\int_0^\pi d\varphi_1 \sin^{d-2}\varphi_1}. \quad \text{(S43)}$$

To calculate the numerator of the right-hand side of Eq. (S43) we use the Poisson integral expression for the Bessel function [16],

$$J_\nu(z) = \frac{\left(\frac{z}{2}\right)^\nu}{\Gamma\left(\nu+\frac{1}{2}\right)\Gamma\left(\frac{1}{2}\right)} \int_0^\pi d\varphi \sin^{2\nu}\varphi e^{iz\cos\varphi} \quad \text{(S44)}$$

for Re$\nu > -\frac{1}{2}$. To calculate the denominator we use the identity [16],

$$\int_0^\pi d\varphi \sin^{\nu-1}\varphi = \frac{\pi}{2^{\nu-1}\nu B\left(\frac{\nu+1}{2}, \frac{\nu+1}{2}\right)} \quad \text{(S45)}$$

for Re$\nu > 0$, where $B(x,y)$ is the beta function. By further using the identity,

$$B(x,x) = 2^{1-2x}B(1/2,x) = 2^{1-2x}\frac{\Gamma(x)\Gamma\left(\frac{1}{2}\right)}{\Gamma\left(x+\frac{1}{2}\right)}, \quad \text{(S46)}$$

we obtain the explicit form of $f$ given by Eq. (4) which was originally given in Ref. 17 albeit without derivations.

## IV. Derivation of Eq. (12)

For two nearest single-particle eigenenergies $\varepsilon, \varepsilon'$, the difference in the arguments of $f$ is

$$|\boldsymbol{r}-\boldsymbol{r}'|\left(\lambda_{\varepsilon'}^{-1} - \lambda_\varepsilon^{-1}\right) \sim \frac{|\boldsymbol{r}-\boldsymbol{r}'|\sqrt{2m\Delta_\varepsilon}}{\hbar}\sqrt{\frac{\Delta_\varepsilon}{\varepsilon}}, \quad \text{(S47)}$$

because the level spacing of local spectrum $\Delta_\varepsilon \ll \varepsilon = \mathcal{O}(E/N)$. Taking into account of the inequalities of $\lambda_\varepsilon \ll L$ and $|\boldsymbol{r}-\boldsymbol{r}'| \lesssim L$ as well as the ergodicity, we obtain

$$\frac{|\boldsymbol{r}-\boldsymbol{r}'|\sqrt{2m\Delta_\varepsilon}}{\hbar}\sqrt{\frac{\Delta_\varepsilon}{\varepsilon}} \sim \frac{|\boldsymbol{r}-\boldsymbol{r}'|}{L}\left(\frac{\lambda_\varepsilon}{L}\right)^{\frac{d-2}{2}}\left(\frac{\Delta_\varepsilon}{\varepsilon}\right)^{\frac{1}{2}} \ll 1. \quad \text{(S48)}$$

Taking the inequalities (S47) and (S48) into account, we obtain Eq. (12).

## V. Time profile of entropy

Basing on the coarse grained Wigner function (S24), we can introduce an entropy defined by Eq. (15). For the convenience we rewrite it below,

$$S(t) \equiv -\iint \frac{d\boldsymbol{q}d\boldsymbol{p}}{(2\pi\hbar)^d}\left(|\tilde{n}|\ln|\tilde{n}| \pm |1\mp\tilde{n}|\ln|1\mp\tilde{n}|\right). \text{(S49)}$$

Note that $\tilde{n} \equiv (2\pi\hbar)^d M_{c.g.}(\boldsymbol{q},\boldsymbol{p};t)$. Below we study its time profile.

First, we consider short times, i.e., $\lambda^{-1} \lesssim t \ll t_E$. In this case it is sufficient to consider initial $M(\boldsymbol{q},\boldsymbol{p};t)$ which is uniform on a compact support with a size much smaller than that of the coarse graining $\chi'$. Because of $t \ll t_E$ Eq. (S30) follows, i.e., the evolution $M(\boldsymbol{q},\boldsymbol{p};t)$ is classical. Although the support of $M(\boldsymbol{q},\boldsymbol{p};t)$ is deformed in the course of time, its (fine grained) value is time independent. The extension of support grows exponentially $\sim e^{\lambda t}$ in the unstable direction. So, upon coarse graining [cf. Eq. (S25)] we smoothen the support. The volume of the ensuing phase space regime, denoted as $\mathcal{A}(t)$, grows exponentially $\sim e^{\lambda t}$. This coarse graining makes $|M(\boldsymbol{q},\boldsymbol{p};t)|$ outside $\mathcal{A}(t)$ significantly small, but not necessarily vanish. Combining with Eq. (S26) and the conservation law,

$$\frac{d}{dt}\iint d\boldsymbol{q}d\boldsymbol{p}\left(G(t)\circ M(0)\right)(\boldsymbol{q},\boldsymbol{p}) = 0, \quad \text{(S50)}$$

this gives the scaling law,

$$M_{c.g.}(\boldsymbol{q},\boldsymbol{p};t) \sim e^{-\lambda t}, \quad \text{(S51)}$$

with the prefactor determined by the initial condition. In deriving Eq. (S51) we used the approximation that $M_{c.g.}(\boldsymbol{q},\boldsymbol{p};t)$ is a constant over the phase space regime $\mathcal{A}(t)$. By using Eqs. (S26) and (S50) we find that $\iint d\boldsymbol{q}d\boldsymbol{p}|M_{c.g.}(\boldsymbol{q},\boldsymbol{p};t)|$ is time independent. Combining with Eq. (S51), this gives

$$S(t) \sim t, \quad \text{for } \lambda^{-1} \lesssim t \ll t_E. \quad \text{(S52)}$$

In derived this equation we used the fact that the second term of Eq. (S49) is exponentially small because of Eq. (S51) and negligible. As we have shown, the linear law (S52) is a result of Lyapunov instability and thereby very general, independent of initial conditions. In Sec. VI we further provide its numerical evidences.

Then, we consider $t \gg t_E$. In this case, from Eqs. (8)-(10) we obtain

$$M_{c.g.}(\boldsymbol{q},\boldsymbol{p};t) = \frac{n(H(\boldsymbol{q},\boldsymbol{p}))}{(2\pi\hbar)^d}. \quad \text{(S53)}$$

With its substitution Eq. (S49) is reduced to

$$S(t) = -\int d\varepsilon\rho\left(n\ln n \pm (1\mp n)\ln(1\mp n)\right), \quad \text{(S54)}$$

where $n(\varepsilon)$ is given by Eq. (14). This is none but the equilibrium Boltzmann entropy [cf. Eq. (4)].

Collecting the asymptotic results of Eqs. (S52) and (S54), we find the time profile of $S(t)$ by smooth extrapolation, as represented by Fig. 1b. Of course, the real behavior of $S(t)$ in intermediate times could be much more complicated and this is far beyond the scope of present work. In addition, even when the system is thermalized ($t \gg t_E$), $S(t)$ can be suppressed from its thermal value due to quantum fluctuations in phase space. The latter causes the suppression of the degree of homogeneity of $M_{c.g.}$. That is, unlike classical statistical mechanics, there is no strict $H$-theorem in quantum mechanics. This was first proven by von Neumann [18] and numerically observed in Ref. [19]. To illustrate this we perform a numerical analysis in the next section.

## VI. Numerical simulation

In this section we provide numerical evidences of the result Eq. (8) and the entropy profile shown in Fig. 1b. To this end we first recall that Eq. (8) is a result of single-particle quantum motion (while many-body aspects enter only into the initial condition of Wigner function). Therefore, we focus on genuine single-particle quantum motion in simulations. Second, we have also shown that Eq. (8) is a result of mixing of classical dynamics as well as volume conservation. Taking these into account we choose a simple model, namely, the quantum baker's map to simulate quantum evolution of Wigner function.

For the precise definition of quantum baker's map we refer to standard literatures (e.g., Ref. [20]). The phase space supporting dynamics of corresponding Wigner function is a two-dimensional torus, with the (dimensionless) coordinates $(q,p) \in [0,1] \times [0,1]$. It is well known [21] that the classical baker's map is mixing and preserves the Lebesgue measure. Owing to its simplicity this (time) discrete map and its variants have been widely used to simulate real chaotic Hamiltonian flow.

For the quantum baker's map the only control parameter is the dimension of Hilbert space $\mathcal{N}$ or, equivalently, the effective Planck's constant $1/(2\pi\mathcal{N})$ [simulating $\hbar/A$ in Eq. (1)]. Note that the highly excited states in chaotic cavities correspond to the eigenstate of quantum baker's map with $\mathcal{N} \gg 1$. For this map the Lyapunov exponent is $\ln 2$ and the Ehrenfest time $t_E = \frac{\ln \mathcal{N}}{\ln 2}$. For simulations we adopt $\mathcal{N} = 960$ for which $t_E \approx 10$. We prepare an initial Wigner function, which is Gaussian centered at $(\frac{1}{3}, \frac{2}{3})$ with a width of 0.05, and simulate its evolution. Figure S2 represents the evolution of coarse grained Wigner function, where the coarse graining factor is Gaussian also, with a width of 0.03. We see that the coarse grained Wigner function becomes uniform over phase space at $t = 10$ which agrees with $t_E$.

To obtain the time profile of entropy we note that the quantum baker's map represents a genuine single-particle quantum motion. Therefore, we slightly modify the definition of entropy as

$$S_b(t) \equiv - \iint dqdp |M_{c.g.}(q,p;t)| \ln |M_{c.g.}(q,p;t)|, \quad \text{(S55)}$$

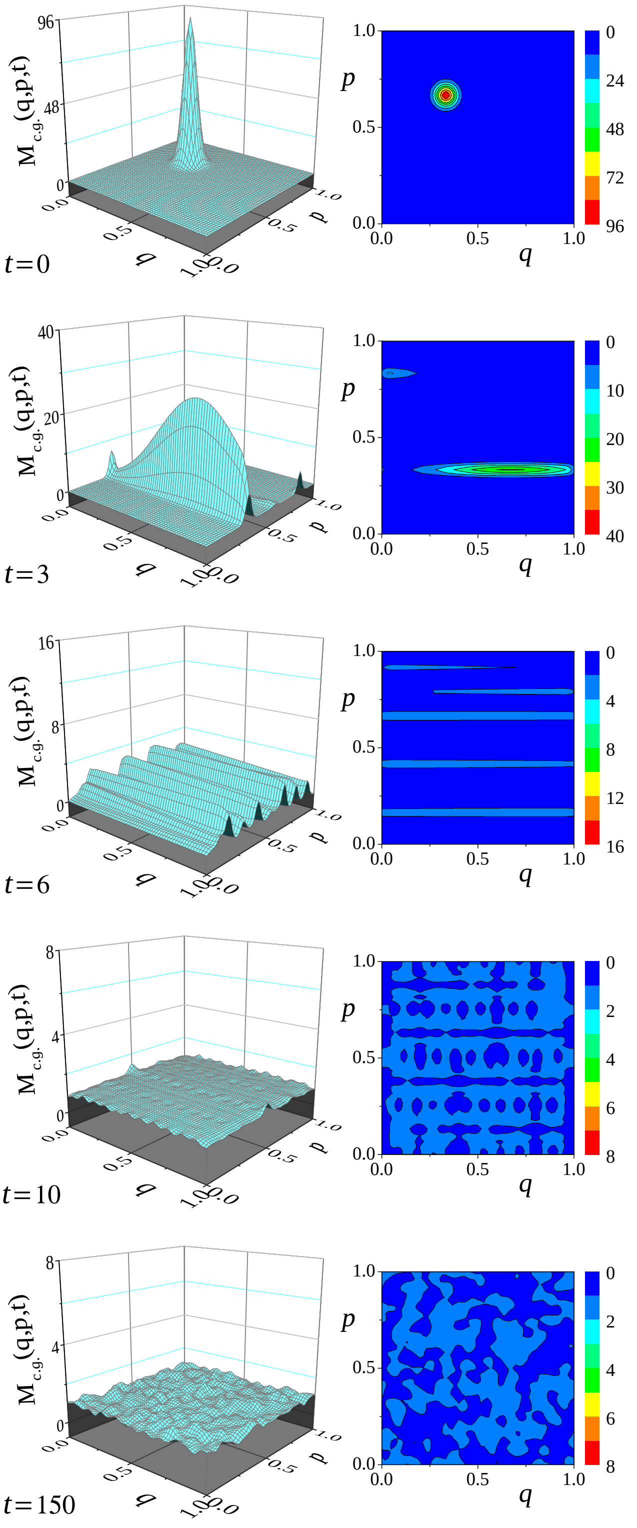


FIG. S2: Representative profiles of Wigner function of quantum baker's map at different stages of evolution. From top to bottom, the time $t = 0, 3, 6, 10$, and 150, respectively. The right column is the corresponding contour plots.

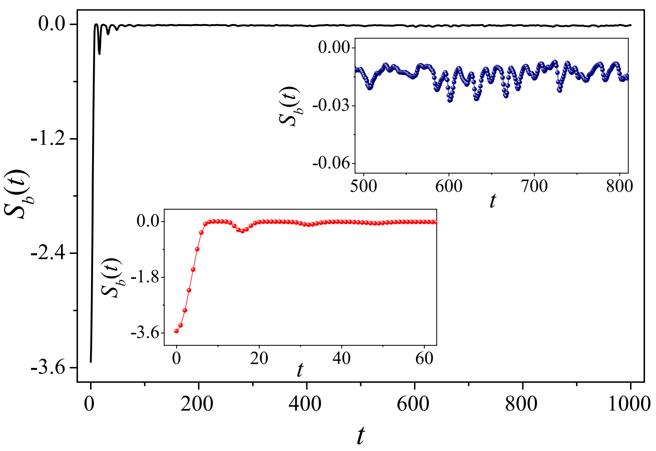


FIG. S3: Simulation results of time profile of entropy for quantum baker's map. Insets: small suppressions of entropy from the upper bound of zero.

where $\iint dqdpM_{c.g.}(q,p;t) = 1$. The simulation results are shown in Fig. S3. As expected the entropy first increases linearly and then saturates. From Fig. S3 we see that $S_b(t) \leq 0$. The upper bound zero corresponds to uniform distribution in phase space. Different from the limiting case of infinite $\mathcal{N}$, where $S_b(t)$ vanishes perfectly in large times, for large but finite $\mathcal{N}$ there are small suppressions in $S(t)$ from time to time (insets). So, there is no strict $H$-theorem in quantum mechanics, as predicted long time ago [18]. These suppressions may be attributed to quantum structures of certain eigenstates.


[1] P. Bocchieri and A. Loinger, Phys. Rev. **107**, 337 (1957).
[2] A. Peres, Phys. Rev. Lett. **49**, 1118 (1982).
[3] M. Hillery, R. F. O'Connell, M. O. Scully, and E. P. Wigner, Phys. Rep. **106**, 121 (1984).
[4] J. E. Moyal, Proc. Cambridge Phil. Soc. **45**, 99 (1949).
[5] A. N. Kolmogorov and S. V. Fomin, *Elements of the Theory of Functions and Functional Analysis*, addendum to Chapter III (Graylock, Rochester, 1963).
[6] C. Beck and F. Schlögl, *Thermodynamics of Chaotic Systems* (Cambridge University Press, Cambridge, UK, 1993).
[7] I. Prigogine, *Nonequilibrium Statistical Mechanics* (Wiley, New York, 1962).
[8] D. Ruelle, Phys. Rev. Lett. **56**, 405 (1986); J. Stat. Phys. **44**, 281 (1986); J. Diff. Geom. **25**, 99 (1987); *ibid.* **25**, 117 (1987).
[9] M. Pollicot, Invent. Math. **81**, 413 (1985).
[10] S. Smale, Bull. Am. Math. Soc. **73**, 747 (1967).
[11] E. J. Heller, Phys. Rev. Lett. **53**, 1515 (1984); in *Les Houches LII, Chaos and Quantum Physics*, edited by M.-J. Giannoni, A. Voros, and J. Zinn-Justin (North-Holland, Amsterdam, 1991).
[12] E. B. Bogomolny, Physica D **31**, 169 (1988).
[13] M. V. Berry, Proc. R. Soc. London Ser. A **423**, 219 (1989); in *Les Houches LII, Chaos and Quantum Physics*, edited by M.-J. Giannoni, A. Voros, and J. Zinn-Justin (North-Holland, Amsterdam, 1991).
[14] C. Manderfeld, J. Phys. A: Math. Gen. **36**, 6379 (2003).
[15] A. P. Prudnikov, Yu. A. Brychkov, and O. I. Marichev, *Integraly i ryady, tom 1. E'lementarnye funkcii* (Nauka, Moscow, 1981).
[16] I. S. Gradshteyn and I.M. Ryzhik, *Tables of Integrals, Series, and Products*, 6th edition (Academic Press, San Diego, 2000).
[17] M. V. Berry, J. Phys.: Math. Gen. A **10**, 2083 (1977).
[18] J. von Neumann, Z. Phys. **57**, 30 (1929).
[19] J. Wang, C.-H. Lai, and Y. Gu, Phys. Rev. E **63**, 056208 (2001).
[20] M. Saraceno, Ann. Phys. **199**, 37 (1990).
[21] J. R. Dorfman, *An introduction to chaos in nonequilibrium statistical mechanics* (Cambridge University Press, Cambridge, UK, 1999).
